# Supplementary material for: PoseDiffusion: Solving Pose Estimation via Diffusion-aided Bundle Adjustment
Source: arXiv:2306.15667 source file (2024-01-24)
Supplement: Supplementary file 1 [file csvs_suppl.tex]

\begin{filecontents}{co3dv2are5.csv}
numframe colmapsift colmapspsg ourswoggs ours relpose
3 0.0815 0.0641 0.1782 0.2937 0.0000
5 0.1408 0.0873 0.2688 0.3589 0.0000
10 0.2366 0.1809 0.3242 0.4991 0.0000
20 0.3989 0.5102 0.3723 0.6627 0.0000
30 0.5098 0.6816 0.3685 0.7064 0.0000
50 0.7382 0.8914 0.3810 0.7576 0.0000
100 0.6554 0.7845 0.3994 0.7859 0.0000
\end{filecontents}

\begin{filecontents}{co3dv2are10.csv}
numframe colmapsift colmapspsg ourswoggs ours relpose
3 0.1555 0.1424 0.3879 0.5462 0.0000
5 0.2251 0.1695 0.5557 0.6407 0.0000
10 0.3206 0.2693 0.6465 0.7421 0.0000
20 0.4788 0.5975 0.6958 0.8245 0.0000
30 0.5888 0.7510 0.6930 0.8304 0.0000
50 0.7701 0.9147 0.7092 0.8479 0.0000
100 0.7042 0.8258 0.7177 0.8656 0.0000
\end{filecontents}

\begin{filecontents}{co3dv2are15.csv}
numframe colmapsift colmapspsg ourswoggs ours relpose
3 0.2198 0.2064 0.5272 0.6605 0.0000
5 0.2918 0.2378 0.6957 0.7483 0.0000
10 0.3792 0.3373 0.7893 0.8266 0.0000
20 0.5369 0.6534 0.8194 0.8786 0.0000
30 0.6380 0.7871 0.8184 0.8752 0.0000
50 0.7905 0.9226 0.8283 0.8851 0.0000
100 0.7442 0.8488 0.8313 0.8958 0.0000
\end{filecontents}

\begin{filecontents}{co3dv2are30.csv}
numframe colmapsift colmapspsg ourswoggs ours relpose
3 0.4018 0.4056 0.7183 0.7985 0.0000
5 0.4724 0.4172 0.8535 0.8674 0.0000
10 0.5290 0.4868 0.9132 0.9216 0.0000
20 0.6613 0.7448 0.9241 0.9445 0.0000
30 0.7461 0.8444 0.9149 0.9280 0.0000
50 0.8372 0.9356 0.9240 0.9326 0.0000
100 0.8090 0.8895 0.9210 0.9422 0.0000
\end{filecontents}

\begin{filecontents}{co3dv2aremean.csv}
numframe colmapsift colmapspsg ourswoggs ours relpose
3 0.3308 0.3269 0.5888 0.6747 0.0000
5 0.3931 0.3392 0.7110 0.7442 0.0000
10 0.4595 0.4154 0.7716 0.8100 0.0000
20 0.5939 0.6791 0.7921 0.8581 0.0000
30 0.6803 0.7925 0.7825 0.8542 0.0000
50 0.8054 0.9120 0.7932 0.8692 0.0000
100 0.7631 0.8500 0.7918 0.8831 0.0000
\end{filecontents}

\begin{filecontents}{co3dv2ate0.1.csv}
numframe colmapsift colmapspsg ourswoggs ours relpose
3 0.0593 0.0635 0.2049 0.2873 0.0000
5 0.0458 0.0124 0.0590 0.1181 0.0000
10 0.0766 0.0348 0.0505 0.1090 0.0000
20 0.1659 0.2066 0.0494 0.1605 0.0000
30 0.2334 0.3425 0.0247 0.1816 0.0000
50 0.3194 0.4379 0.0242 0.2324 0.0000
100 0.4072 0.4800 0.0250 0.2752 0.0000
\end{filecontents}

\begin{filecontents}{co3dv2ate0.25.csv}
numframe colmapsift colmapspsg ourswoggs ours relpose
3 0.0846 0.0939 0.3832 0.4795 0.0000
5 0.0879 0.0445 0.1692 0.2786 0.0000
10 0.1403 0.0986 0.1349 0.2957 0.0000
20 0.2670 0.3567 0.1245 0.3977 0.0000
30 0.3462 0.5256 0.1039 0.4423 0.0000
50 0.4515 0.6359 0.1031 0.5076 0.0000
100 0.5301 0.6734 0.1060 0.5582 0.0000
\end{filecontents}

\begin{filecontents}{co3dv2ate0.5.csv}
numframe colmapsift colmapspsg ourswoggs ours relpose
3 0.1150 0.1201 0.5863 0.6491 0.0000
5 0.1170 0.0651 0.3705 0.4945 0.0000
10 0.1837 0.1406 0.3206 0.5134 0.0000
20 0.3268 0.4342 0.3158 0.6048 0.0000
30 0.4237 0.6185 0.2924 0.6405 0.0000
50 0.5249 0.7286 0.2951 0.6907 0.0000
100 0.5924 0.7573 0.2991 0.7238 0.0000
\end{filecontents}

\begin{filecontents}{co3dv2ate1.0.csv}
numframe colmapsift colmapspsg ourswoggs ours relpose
3 0.1525 0.1446 0.7660 0.7976 0.0000
5 0.1535 0.0902 0.6367 0.6989 0.0000
10 0.2204 0.1733 0.5944 0.7057 0.0000
20 0.3805 0.4980 0.6050 0.7621 0.0000
30 0.4788 0.6774 0.5901 0.7753 0.0000
50 0.5820 0.7784 0.6001 0.8036 0.0000
100 0.6401 0.7995 0.6101 0.8229 0.0000
\end{filecontents}

\begin{filecontents}{co3dv2atemean.csv}
numframe colmapsift colmapspsg ourswoggs ours relpose
3 0.2714 0.2505 0.8400 0.8634 0.0000
5 0.2513 0.1900 0.7559 0.7854 0.0000
10 0.2846 0.2477 0.7381 0.7827 0.0000
20 0.4514 0.5693 0.7498 0.8205 0.0000
30 0.5457 0.7188 0.7336 0.8148 0.0000
50 0.6393 0.7937 0.7412 0.8346 0.0000
100 0.6783 0.8110 0.7447 0.8454 0.0000
\end{filecontents}

\begin{filecontents}{co3dv2rre5.csv}
numframe colmapsift colmapspsg ourswoggs ours relpose
3 0.1074 0.1608 0.2950 0.4230 0.0000
5 0.1704 0.1515 0.3319 0.4690 0.0000
10 0.2626 0.2614 0.3743 0.5889 0.0000
20 0.5144 0.6791 0.4005 0.7080 0.0000
30 0.6208 0.8058 0.3903 0.7474 0.0000
50 0.7147 0.8613 0.4065 0.7975 0.0000
100 0.7897 0.8736 0.4227 0.8339 0.0000
\end{filecontents}

\begin{filecontents}{co3dv2rre10.csv}
numframe colmapsift colmapspsg ourswoggs ours relpose
3 0.1597 0.2076 0.5675 0.6244 0.0000
5 0.2107 0.1855 0.6256 0.6873 0.0000
10 0.3013 0.2926 0.6806 0.7830 0.0000
20 0.5421 0.6993 0.7110 0.8470 0.0000
30 0.6447 0.8216 0.7043 0.8564 0.0000
50 0.7369 0.8747 0.7212 0.8835 0.0000
100 0.8091 0.8857 0.7345 0.8987 0.0000
\end{filecontents}

\begin{filecontents}{co3dv2rre15.csv}
numframe colmapsift colmapspsg ourswoggs ours relpose
3 0.2005 0.2328 0.7079 0.7383 0.0000
5 0.2482 0.2119 0.7628 0.7926 0.0000
10 0.3311 0.3164 0.8120 0.8539 0.0000
20 0.5594 0.7070 0.8403 0.8960 0.0000
30 0.6586 0.8275 0.8326 0.8933 0.0000
50 0.7475 0.8793 0.8413 0.9105 0.0000
100 0.8184 0.8900 0.8521 0.9193 0.0000
\end{filecontents}

\begin{filecontents}{co3dv2rre30.csv}
numframe colmapsift colmapspsg ourswoggs ours relpose
3 0.2846 0.2840 0.8333 0.8437 0.0000
5 0.3335 0.2737 0.8785 0.8837 0.0000
10 0.4071 0.3764 0.9118 0.9152 0.0000
20 0.5990 0.7210 0.9327 0.9423 0.0000
30 0.6866 0.8359 0.9227 0.9285 0.0000
50 0.7690 0.8862 0.9275 0.9387 0.0000
100 0.8346 0.8971 0.9334 0.9426 0.0000
\end{filecontents}

\begin{filecontents}{co3dv2rremean.csv}
numframe colmapsift colmapspsg ourswoggs ours relpose
3 0.2462 0.2521 0.7006 0.7321 0.0000
5 0.2937 0.2440 0.7415 0.7741 0.0000
10 0.3706 0.3464 0.7782 0.8243 0.0000
20 0.5715 0.6990 0.8006 0.8678 0.0000
30 0.6613 0.8152 0.7902 0.8647 0.0000
50 0.7457 0.8667 0.7973 0.8840 0.0000
100 0.8126 0.8782 0.8053 0.8952 0.0000
\end{filecontents}

\begin{filecontents}{co3dv2rte5.csv}
numframe colmapsift colmapspsg ourswoggs ours relpose
3 0.0332 0.0734 0.2723 0.4487 0.0000
5 0.0856 0.0717 0.3119 0.5140 0.0000
10 0.1736 0.1737 0.3422 0.6109 0.0000
20 0.4080 0.5723 0.3651 0.7056 0.0000
30 0.5130 0.7008 0.3513 0.7257 0.0000
50 0.6162 0.7669 0.3629 0.7628 0.0000
100 0.6957 0.7847 0.3755 0.7841 0.0000
\end{filecontents}

\begin{filecontents}{co3dv2rte10.csv}
numframe colmapsift colmapspsg ourswoggs ours relpose
3 0.0558 0.1150 0.5109 0.6658 0.0000
5 0.1133 0.1017 0.5627 0.7191 0.0000
10 0.2052 0.2109 0.6050 0.7794 0.0000
20 0.4607 0.6337 0.6302 0.8300 0.0000
30 0.5701 0.7588 0.6208 0.8288 0.0000
50 0.6729 0.8192 0.6309 0.8470 0.0000
100 0.7486 0.8324 0.6413 0.8590 0.0000
\end{filecontents}

\begin{filecontents}{co3dv2rte15.csv}
numframe colmapsift colmapspsg ourswoggs ours relpose
3 0.0721 0.1442 0.6420 0.7508 0.0000
5 0.1285 0.1168 0.6881 0.7937 0.0000
10 0.2198 0.2260 0.7281 0.8373 0.0000
20 0.4867 0.6594 0.7519 0.8744 0.0000
30 0.5999 0.7825 0.7420 0.8659 0.0000
50 0.7012 0.8393 0.7493 0.8794 0.0000
100 0.7739 0.8514 0.7575 0.8881 0.0000
\end{filecontents}

\begin{filecontents}{co3dv2rte30.csv}
numframe colmapsift colmapspsg ourswoggs ours relpose
3 0.1023 0.1949 0.7883 0.8390 0.0000
5 0.1537 0.1443 0.8244 0.8684 0.0000
10 0.2404 0.2510 0.8566 0.8987 0.0000
20 0.5345 0.7028 0.8788 0.9247 0.0000
30 0.6573 0.8184 0.8661 0.9110 0.0000
50 0.7526 0.8683 0.8707 0.9202 0.0000
100 0.8179 0.8784 0.8757 0.9254 0.0000
\end{filecontents}

\begin{filecontents}{co3dv2rtemean.csv}
numframe colmapsift colmapspsg ourswoggs ours relpose
3 0.0852 0.1687 0.6636 0.7411 0.0000
5 0.1353 0.1257 0.6993 0.7752 0.0000
10 0.2205 0.2291 0.7298 0.8156 0.0000
20 0.4979 0.6609 0.7504 0.8537 0.0000
30 0.6158 0.7767 0.7372 0.8467 0.0000
50 0.7108 0.8289 0.7429 0.8620 0.0000
100 0.7779 0.8410 0.7490 0.8713 0.0000
\end{filecontents}
